# Supplementary material for: Robust Graph Learning Under Wasserstein Uncertainty
Source: arXiv:2105.04210 source file (2021-05-13)
Supplement: Supplementary file 1 [file appendix4.tex]

We first prove that $g(\gamma,\mathbf{L})$ is convex respect to $\gamma$. As stated in (\ref{derivative with gamma}), the derivative of $g(\gamma,\mathbf{L})$ with $\gamma$ is 
\begin{equation}
    \begin{aligned}
    \frac{\partial g (\gamma,\mathbf{L})}{\partial \gamma} = \epsilon^2 -  \parallel \bm{\mu}_n - \gamma (\gamma \mathbf{I} - \mathbf{L})^{-1}\bm{\mu}_n \parallel_2^2 - \text{Tr}\left[\mathbf{\Sigma}_n(\mathbf{I}-\gamma(\gamma\mathbf{I}-\mathbf{L})^{-1})^2\right].\label{derivative with gamma-1}
    \end{aligned}
\end{equation}

We further calculate the second derivative as follows, 
\begin{equation}
    \begin{aligned}
    \frac{\partial g^2 (\gamma,\mathbf{L})}{\partial \gamma^2} = 2\text{Tr}\left((\mathbf{I} - \gamma(\gamma\mathbf{I} - \mathbf{L})^{-1})^2 (\gamma\mathbf{I}-\mathbf{L})^{-1}\right)
        \label{second derivative with gamma}
    \end{aligned}
\end{equation}
Since $\gamma\mathbf{I} \succ \mathbf{L}$, $ \frac{\partial g^2 (\gamma,\mathbf{L})}{\partial \gamma^2} \geq 0 $, and we can conclude that $g(\gamma,\mathbf{L})$ is convex respect to $\gamma$.
Next, we fix $\gamma$ and the problem boils down to (\ref{reformulation-update L}). It is apparently that the objective function and constraints are all convex. Therefore, $g(\gamma,\mathbf{L})$ is convex respect to $\mathbf{L}$.

From above analysis, we can reach the conclusion that $g(\gamma,\mathbf{L})$ is convex respect to $\gamma$ and $\mathbf{L}$ separeately.
